# Supplementary material for: Grimm in Wonderland: Prompt Engineering with Midjourney to Illustrate Fairytales
Source: arXiv:2302.08961 source file (2023-08-25)
Supplement: Supplementary file 1 [file tab-appendix2-failure.tex]

% table
% - prompt
% - results
% - comment

Cinderella... went to her mother's grave, and planted the branch on it.

Then Gretel gave [the witch] a shove, causing her to fall in

of scissors
and began to cut open the wolf’s belly

\begin{table}[!htbp]%[!ht]
\centering
\resizebox{\columnwidth}{!}{
\begin{tabularx}{\textwidth}{XXp{0.03\textwidth}c}
\hline
    \textbf{Original Text} & \textbf{Complete Prompt} & \textbf{Stage} & \textbf{Image} \\
\hline
faithful Johannes, who was sitting at the front of the ship... saw three ravens flying through the air towards them
 &
three ravens flying by a frigate in open sea, simple book illustration
 &
3
 &
\raisebox{-\totalheight/2}{\includegraphics[width=0.24\textwidth]{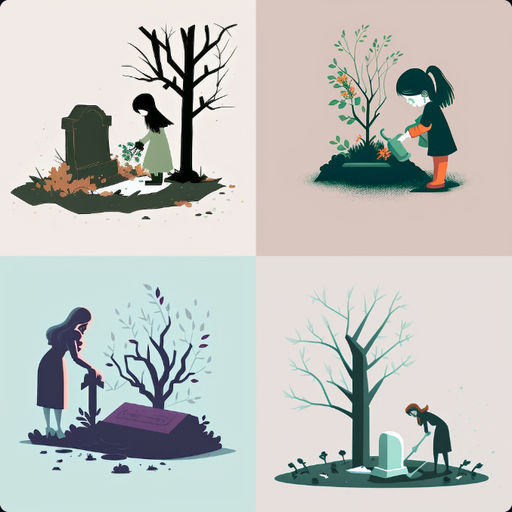}}
 \\
faithful Johannes, who was sitting at the front of the ship... saw three ravens flying through the air towards them
 &
three ravens flying by a frigate in open sea, simple book illustration
 &
1
 &
\raisebox{-\totalheight/2}{\includegraphics[width=0.24\textwidth]{images/fig4-hansel-shove.png}}
 \\
faithful Johannes, who was sitting at the front of the ship... saw three ravens flying through the air towards them
 &
three ravens flying by a frigate in open sea, simple book illustration
 &
2
 &
\raisebox{-\totalheight/2}{\includegraphics[width=0.24\textwidth]{images/fig4-redcap-cut.png}}
\end{tabularx}
}
\caption{Further examples Samples from all stages that led up to the results in Table~\ref{tab:samples-failure}.}
\label{tab:appendix-failure}
\end{table}
